# Supplementary material for: Embedding-based Zero-shot Retrieval through Query Generation
Source: arXiv:2009.10270 source file (2020-09-22)
Supplement: Supplementary file 1 [file appendix.tex]

\appendix

\section{Experiment on ReQA}\label{sec:appendix}
Retrieval Question-Answering (ReQA) is a benchmark for evaluating large-scale sentence-level answer retrieval models introduced by \cite{ahmad2019reqa}. ReQA benchmark is created from the official SQuAD and Natural Questions datasets. The setup of ReQA is different from the standard passage retrieval task. In ReQA, the candidate is a sentence concatenated with its passage that contains the sentence. The goal is to retrieval the correct answer sentence along with its right context passage. Specifically, for each regular passage  of $k$ sentences $P = [s_1,\cdots, s_k]$, it will generate $k$ candidates $(s_1, P), \cdots, (s_k, P)$. To avoid confusion, we call these concatenated passages as candidates. We use the ReQA code\footnote{https://github.com/ google/retrieval-qa-eval} to process the SQuAD and Nature Questions datasets. The details of the processed datasets are shown in \cref{table:reqadataset}.

\begin{table}[ht]
\begin{minipage}{1.0\linewidth}
	\centering
	\footnotesize
\begin{tabu}{@{}lcc@{}}
\toprule
              & SQuAD (ReQA) & Natural Questions (ReQA) \\
\midrule
\# Questions  & 87,599       & 74,097                   \\
\# Passages   & 18,896       & 58,699                   \\
\# Candidates & 91,707       & 239,013                  \\
\bottomrule
\end{tabu}
\end{minipage}
\caption{Summary of the ReQA datasets.}
\label{table:reqadataset}
\end{table}

We first benchmark the two datasets using BM25 from eleasticsearch with default settings and also evaluate the Two-Tower and Siamese models pretrained on WikiGQ dataset on these datasets as well. The results are shown in 
\cref{table:squadreqa} and \ref{table:nqreqa}.
\begin{table*}[ht]
\begin{minipage}{1.0\linewidth}
	\centering
	\footnotesize
\begin{tabu}{@{}l|l|ccccc@{}}
\toprule
\textbf{Model}    & \textbf{Pretraining} & \textbf{R@1}   & \textbf{R@5}   & \textbf{R@10}  & \textbf{R@50}  & \textbf{R@100} \\
\midrule
USE-QA \cite{ahmad2019reqa}   & -           & 43.9  & 65.6  & 72.7  &  -    & -    \\
% BM25 \cite{chang2020pre}      & -           & 41.86 & 58.00 & 63.64 & 74.15 & 77.91 \\
Two-Tower \cite{chang2020pre} & ICT+BFS+WLP & 37.43 & 61.48 & 70.18 & 85.37 & 89.85 \\
\midrule
BM25  & -           & \textbf{58.51} & \textbf{76.80} & \textbf{82.14} & 90.45 & 92.72 \\
Two-Tower & WikiGQ      & 41.29 & 67.59 & 76.03 & 89.10 & 92.51 \\
Siamese   & WikiGQ      & 46.53 & 72.52 & 80.27 & \textbf{91.42} & \textbf{94.19} \\
\bottomrule
\end{tabu}
\end{minipage}
\caption{Zero-short Performance on SQuAD ReQA dataset. Since \cite{chang2020pre} did not report zero-shot performance, we report their numbers with $1\%/99\%$ training/test split setting (same for the Natural questions dataset.}.
\label{table:squadreqa}
\end{table*}

\begin{table*}[ht]
\begin{minipage}{1.0\linewidth}
	\centering
	\footnotesize
\begin{tabu}{@{}l|l|ccccc@{}}
\toprule
\textbf{Model}     & \textbf{Pretraining} & \textbf{R@1}   & \textbf{R@5}   & \textbf{R@10}  & \textbf{R@50}  & \textbf{R@100} \\
\midrule
USE-QA \cite{ahmad2019reqa}.  & -           & 14.7  & 31.7  & 39.1  & -     & -     \\
% BM25 \cite{chang2020pre}      & -           & 4.99  & 11.91 & 15.41 & 24.00 & 27.97 \\
Two-Tower \cite{chang2020pre} & ICT+BFS+WLP & 17.31 & 43.62 & 55.00 & 76.59 & 82.84 \\
\midrule
BM25  & -           & 18.06 & 42.23 & 52.26 & 70.71 & 76.52 \\
Two-Tower & WikiGQ      & 21.71 & 55.55 & 68.35 & 86.65 & 90.83 \\
Siamese   & WikiGQ      & \textbf{21.88} & \textbf{56.48} & \textbf{69.67} & \textbf{87.93} & \textbf{91.88} \\
\bottomrule
\end{tabu}
\end{minipage}
\caption{Zero-short Performance on Natural Questions ReQA dataset.}
\label{table:nqreqa}
\end{table*}
